# Supplementary material for: Detecting structured sources in noisy images via Minkowski maps
Source: arXiv:2111.13348 ancillary file (2021-11-26)
Supplement: Supplementary file 1 [file minkowski-maps-supplementary-material.pdf]

# Supplementary Material: Detecting structured sources in noisy images via Minkowski maps

MICHAEL A. KLATT<sup>1</sup> and KLAUS MECKE<sup>2</sup>

<sup>1</sup> *Department of Physics, Princeton University, Princeton, NJ 08544, USA*

<sup>2</sup> *Institut für Theoretische Physik, FAU Erlangen-Nürnberg, Staudtstr. 7, 91058 Erlangen, Germany*

PACS 07.05.Kf – Data analysis: algorithms and implementation; data management

PACS 02.50.-r – Probability theory, stochastic processes, and statistics

PACS 02.40.-k – Geometry, differential geometry, and topology

**Minkowski functionals.** – Minkowski functionals have been successfully applied in many fields of science, including physics [1,2], biology [3,4], mathematics [5], stereology [6], material sciences [7,8], medical imaging [9], and pattern analysis [10].

In 2D, the Minkowski functionals of a compact body  $K$ , such as the collection of black pixels within the observation window, are the area  $A$ , perimeter  $P$ , and Euler characteristic  $\chi$ . The latter is a topological constant given by the number of connected components (clusters) minus the number of holes (cavities). Their integral representations for a smooth body  $K$  are:

$$A = \int_K dA, \quad P = \int_{\partial K} dl, \quad \text{and} \quad \chi = \int_{\partial K} \frac{\kappa}{2\pi} dl \quad (1)$$

where  $\kappa$  is the curvature. For the rich mathematical background, see, e.g., ref. [5].

Intuitive introductions for applied scientists are provided elsewhere [7,11,12]. The website

<https://morphometry.org>

offers besides a section on the theory of Minkowski functionals (and their generalization to tensors) also a software tool for hands-on experience and image analysis via Minkowski tensors.

Here we quantify the structure of pixelated gray-scale images. To this end the original image data is first turned into a black-and-white (b/w) image via thresholding, that is, all pixels with a greyscale larger or equal a given threshold  $\rho$  are set to black (otherwise white).

**Density of states.** – The density of states  $\Omega$  is the number of b/w images (microstates) with the same area, perimeter, and Euler characteristic (macrostate). By combining analytical and numerical results, as explained in the main text, we achieve an accurate estimate of  $\Omega$  and thus

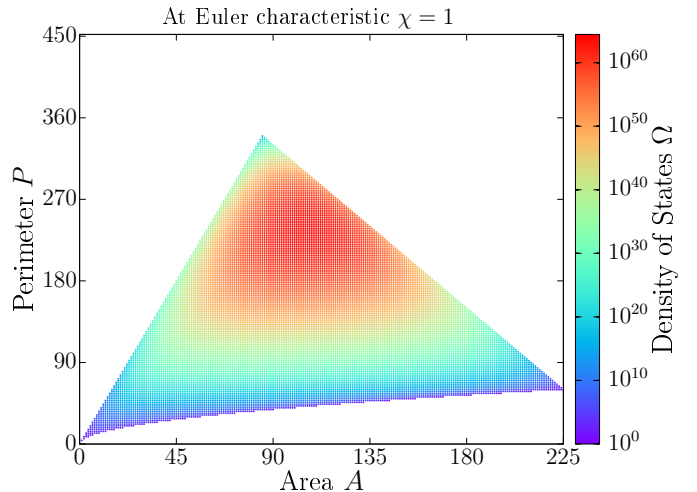

Fig. 1: Density of states  $\Omega$  of macrostates with  $\chi = 1$  for all possible values of  $A$  and  $P$  accurately estimated for a window of  $15 \times 15$  pixels. The color scale represents the values of  $\Omega$ . They range over 64 orders of magnitude.

of the joint probability distribution  $\mathcal{P}(\mathcal{A}, \mathcal{P}, \chi)$  of the three Minkowski functionals. The latter is exactly normalized.

Figure 1 shows an exemplary result, where  $\Omega$  varies over 64 orders of magnitude. The figure plots a “slice” of the DoS, that is, for a fixed value of the Euler characteristic the plot shows the DoS for all possible values of area  $A$  and perimeter  $P$ . There are three obvious constraints on the latter. The smallest perimeter  $P$  for a given area  $A$  and Euler characteristics  $\chi = 1$  is attained by an approximation of a disc. The two approximately linear constraints—on the maximal perimeter (given  $A$  and  $\chi$ )—correspond to checkerboard-like configurations. The constraints change with  $\chi$ , as can be seen in the supplementary animations.

There, the “slices” at fixed values of the Euler characteristic  $\chi$  scan all allowed values of  $\chi$  for b/w images with  $7 \times 7$  or  $15 \times 15$  pixels.

**Detector acceptance correction.** – Observations in gamma-ray astronomy are typically affected by a spatially varying detector acceptance, that is, for each bin  $i$  only a fraction  $f_i$  of the signals are detected on average. Using a model for the camera acceptance, we can take such detector effects into account when we analyze real data.

We first present a basic technique that regains an isotropic and homogeneous structure for background measurements via Monte Carlo observations [11]. It is complemented by the possibility to subtract point sources via postselection. Both techniques are then combined to obtain a slightly improved detector acceptance correction. Finally, we extend this concept to an optimal correction. It adjusts the analysis to the variations in the acceptance locally, resulting in a minimal suppression of source signals. These corrections make it possible to adjust our morphometric analysis to typical requirements of measurements.

In a simulation study, in fig. 2, we explicitly demonstrate the correction of a strongly inhomogeneous detector acceptance. Figures 2 (d–f) are Minkowski maps based on the area, the perimeter, and the Euler characteristic (for a sliding window size  $6 \times 6$ ). They analyze the counts map in fig. (c) corrected by the three different techniques mentioned above and explained below. To show the reliability of our approach independent of fluctuations in a single example, we average 100 of such Minkowski maps in figs. 2 (g–i), which can, of course, not be directly used in a null hypothesis test.

The basic technique has already been sufficient to analyze the experimental gamma-ray sky map measured by H.E.S.S., see fig. 5 in the main text. Our new, advanced local detector correction detects sources even at the faint edge of the observation window, where the signals are hardly visible by eye compared to the strong signal in the central field of view.

*Monte Carlo observations.* As an example, we choose in fig. 2(a) a detector acceptance that is Gaussian-shaped with  $f_i = 1$  in the center of the sky map. The black line indicates the line of half-maximum. A counts map is first simulated at a homogeneous Poisson background with intensity 100 and nine differently strong sources are placed at different distances to the center, see fig. 2(b). Then, for each pixel, only a fraction  $f_i$  of the counts are accepted according to fig. 2(a). The resulting counts map is depicted in fig. 2(c).

If the counts in pixel  $i$  with acceptance  $f_i$  were naively weighted with  $1/f_i$ , fractional counts would appear, resulting in a non-Poisson structure of the sky map. To correct the acceptance and regain a homogeneous Poisson counts maps, we instead use the null hypothesis that the background signals form a homogeneous Poisson process with intensity  $\lambda$ . The detected number of counts in

bin  $i$  is therefore assumed to be a Poisson random variable with mean value  $\lambda_i = f_i \lambda$ . So we add to it a new Poisson-distributed random variable, that is, Monte Carlo observations, with mean value  $\lambda_i^+ = (1 - f_i) \lambda$ .

Therefore, the sum is a new random variable with mean value  $\lambda$ . Under the null hypothesis, we obtain a homogeneous background noise. The sums of measured counts and pseudo-photon counts from the Monte Carlo observations fulfill the null hypothesis by construction. So they do not introduce additional structural deviations from the homogeneous isotropic Poisson field.

If  $f_i \approx 1$  (typically in the center of the field of view), the number of counts is nearly unchanged. However, source features in regions where  $f_i \ll 1$  are covered by the additionally created pseudo-photon counts. So the correction is conservative.

In figs. 2(d) and 2(g), the entire counts map is corrected by adding Monte Carlo observations up to intensity  $\lambda$ . Only the central source is clearly visible. The other source signals are overwhelmed by the additional simulated Poisson signals.

*Postselection.* If there is a strong pointlike source within the field of view, it needs to be subtracted from the data to detect diffuse gamma-ray signals, that is, extended sources in the same field of view (like in Ref. [13]). As for the acceptance correction above, a simple multiplication with a non-integer factor is not appropriate. Postselection offers a convenient and efficient solution.

First, we formulate a new null hypothesis that there is no additional source besides the known source that is to be subtracted. It implies that the number of counts in bin  $i$  is a Poisson random variable with mean value  $\lambda + \Lambda_i$ , where  $\lambda$  is the intensity of the background and  $\Lambda_i$  the contribution of the pointlike source.

On average, the number of counts has to be reduced by a factor of  $\lambda/(\lambda + \Lambda_i)$ . We maintain the integer number of counts by a Monte Carlo postselection of the events. Only  $n$  of the  $k$  signals that have been recorded in bin  $i$  are kept. This number  $n$  follows a Binomial distribution with probability  $\lambda/(\lambda + \Lambda_i)$  resulting in a homogeneous Poisson counts map with intensity  $\lambda$ . The estimate is conservative and thus stable against errors in the model of the pointlike source [14].

*Combined postselection and MC observations.* As mentioned above, the detector acceptance correction by Monte Carlo observations is conservative in regions of very low acceptance  $f_i \ll 1$ . The additional Poisson random number suppresses the detection of an excess or structural deviation in the actual counts, for example, if Monte Carlo observations and measured signals differ by an order of magnitude.

This unbalance can be avoided by combining the Monte Carlo observations and postselection [15, 16]. Instead of the original expected intensity  $\lambda$ , their target intensity is chosen to be  $f \lambda$ , where  $f$  is between the maximum and minimum acceptance. For bins with  $f_i < f$ , MC obser-

vations are added to the data set [on average  $(f - f_i)\lambda$  events]. For bins with  $f_i > f$ , the signals are reduced via the postselection as described above [on average by a factor of  $f/f_i$ ].

The method can be optimized for a region of interest, by setting  $f$  to the corresponding acceptance  $f_j$  in this region. A nearly optimal detector acceptance correction can thus be achieved for a limited region with  $f_i \approx f_j$ .

In figs. 2(e) and 2(h), a target intensity  $\lambda/2$  is chosen, and a homogeneous Poisson field is regained under the null hypothesis via both Monte Carlo observations and postselection. The four sources in the region of the target intensity are clearly visible. The sources in the corners and the central sources are sometimes detected depending on the strong fluctuations at a low number of counts.

*Local detector acceptance correction.* To avoid conservative estimates in the entire observation window, the value of  $f_j$  has to be adopted locally. Instead of correcting the detector acceptance globally and prior to the construction of the Minkowski map, it is performed separately and independently for each position of the sliding window. The increase in computation time is recompensed by a tremendous increase in sensitivity that can be achieved by such a local detector acceptance compared to the global acceptance correction described above.

Given the acceptance  $f_i$  of the central bin of a sliding window, the target intensity is chosen to be  $f_i\lambda$ , and the original observed counts map is corrected by the combined postselection and MC observation. Thus, we perform an optimal acceptance correction for each sliding window. An additional advantage is that the correlation between overlapping observation windows slightly decreases (due to the different random variables of the postselection and MC observation).

The hypothesis test is performed for each pixel in the Minkowski map at a different background intensity. Since the probability that a pixel is black at a given threshold varies between sliding windows, the probability distribution  $\mathcal{P}(A, P, \chi)$  from Eq. (1) in the main text has to be determined separately for each pixel in the Minkowski map. The resulting increase in computation time (compared to the former fast detector acceptance corrections with a global background intensity) is justified by a strong increase in sensitivity whenever weak sources ought to be detected despite strong detector effects.

The tremendous gain in sensitivity is demonstrated in Figs. 2(f) and 2(i). In a single Minkowski map, our advanced background correction reliably detects all sources at any distance to the center.

## REFERENCES

- [1] MECKE K., *Int. J. Mod. Phys. B*, **12** (1998) 861.
- [2] MECKE K. and STOYAN D., *Statistical Physics and Spatial Statistics - The Art of Analyzing and Modeling Spatial Structures and Pattern Formation* 1st Edition Vol. 554 of *Lecture Notes in Physics* (Springer, Berlin) 2000.
- [3] BEISBART C., BARBOSA M. S., WAGNER H. and COSTA L. D. F., *Eur. Phys. J. B*, **52** (2006) 531.
- [4] BARBOSA M., NATOLI R., VALTER K., PROVIS J. and MADDESS T., *Biomed. Opt. Express*, **5** (2014) 2317.
- [5] SCHNEIDER R. and WEIL W., *Stochastic and Integral Geometry (Probability and Its Applications)* (Springer, Berlin) 2008.
- [6] LEGLAND D., KIÉU K. and DEVAUX M.-F., *Image Analysis & Stereology*, **26** (2011) 83.
- [7] SCHRÖDER-TURK G. E. *et al.*, *Adv. Mater.*, **23** (2011) 2535.
- [8] OHSEER J. and SCHLADITZ K., *3D images of materials structures: processing and analysis* (Wiley-VCH, Weinheim) 2009.
- [9] RÄTH C., MONETTI R., BAUER J., SIDORENKO I., MÜLLER D., MATSUURA M., LOCHMÜLLER E. M., ZYSSET P. and ECKSTEIN F., *New J. Phys.*, **10** (2008) 125010.
- [10] MANTZ H., JACOBS K. and MECKE K., *J. Stat. Mech.*, **12** (2008) P12015.
- [11] GÖRING D., KLATT M. A., STEGMANN C. and MECKE K., *Astron. Astrophys.*, **555** (2013) A38.
- [12] KLATT M. A., SCHRÖDER-TURK G. E. and MECKE K., *Med. Phys.*, **44** (2017) 3663.
- [13] AHARONIAN F. *et al.*, *Nature*, **439** (2006) 695.
- [14] KLATT M. A., *Morphometric analysis in gamma-ray astronomy* Master's thesis (Diplomarbeit) Universität Erlangen-Nürnberg (2010).
- [15] GÖRING D., *Gamma-Ray Astronomy Data Analysis Framework based on the Quantification of Background Morphologies using Minkowski Tensors* Ph.D. thesis Universität Erlangen-Nürnberg (2012).
- [16] KLATT M. A., *Morphometry of random spatial structures in physics* Ph.D. thesis Friedrich-Alexander-Universität Erlangen-Nürnberg (FAU). (2016).

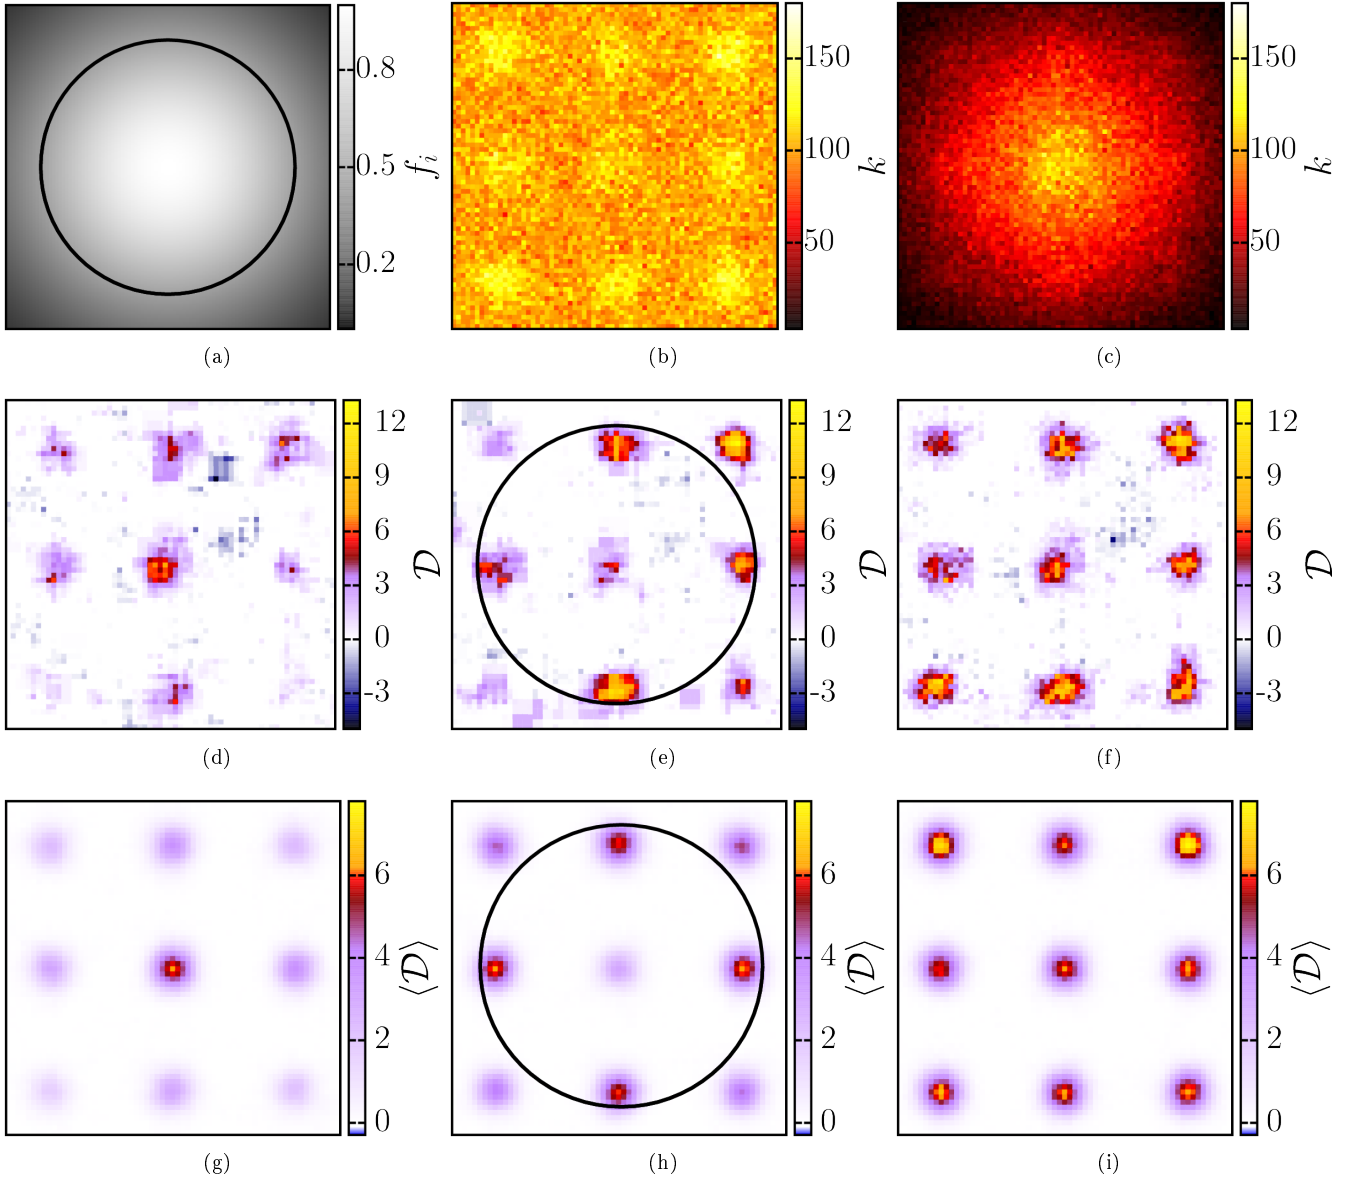

Fig. 2: Detector acceptance correction: (a) acceptance map  $f_i$ ; (b) unreduced simulated counts map; (c) counts are randomly reduced according to acceptance map; (d-f) Minkowski maps analyzing the counts map depicted in (c) for which the acceptance is corrected by our three different methods: (d) globally via Monte Carlo observations; (e) a combination with postselection, where the region of interest that corresponds to the target intensity  $\lambda/2$  is indicated by a black circle; (f) locally. Using the local correction in (f), a single Minkowski sky map detects all sources at any distance to the center. Subfigures (g-i) represent a systematic study. Each pixel shows the average over 100 Minkowski maps, where the acceptance is corrected by the methods used in (d-f).
